# Supplementary material for: Thermal conductivity of strong coupling V$_{1-x}$Ti$_x$ superconductors in the Mott-Ioffe-Regel limit
Source: arXiv:1810.02083 source file (2018-10-04)
Supplement: Supplementary file 1 [file Supplementary_materials.pdf]

# Supplementary materials

## ❖ Sample preparation:

To prepare the $V_{1-x}Ti_x$ alloys (x = 0, 0.1, 0.3, 0.5, 0.6) pure V (99.8 %, Sigma-Aldrich) and pure Ti (99.99 %, Alfa Aesar) were taken in atomic proportions and melted together on a water-cooled copper hearth of a tri-arc-melting furnace in pure Ar-atmosphere. Button like samples were obtained after the melting. The samples were flipped and re-melted five times to ensure homogeneity. The samples were further cut and shaped in different sizes and shapes for various measurements. For the thermal conductivity measurement, samples were cut in rectangular shape having dimensions of about 10 mm×2 mm×2mm.

## ❖ X-ray diffraction analysis:

The room temperature X-ray diffraction (XRD) measurements for the $V_{1-x}Ti_x$ alloys were done in a Bruker D8 Advance diffractometer. Figure 1 shows the XRD patterns of these alloys. The XRD patterns of all the samples show sharp peaks. We found that the samples have formed in the body centred cubic phase which is commensurate with the literature [1-2]. The two peaks marked by '*' which appear at the same positions in all the samples are due to the contribution from the sample holder. Absence of any other peak indicates that no secondary phase is present in the samples. Lattice parameter has been estimated for all the samples. Figure 2 shows the variation of lattice parameters of the $V_{1-x}Ti_x$ alloys as a function of the Ti-concentration. The lattice parameter varies almost linearly with increasing Ti-content for these alloys.

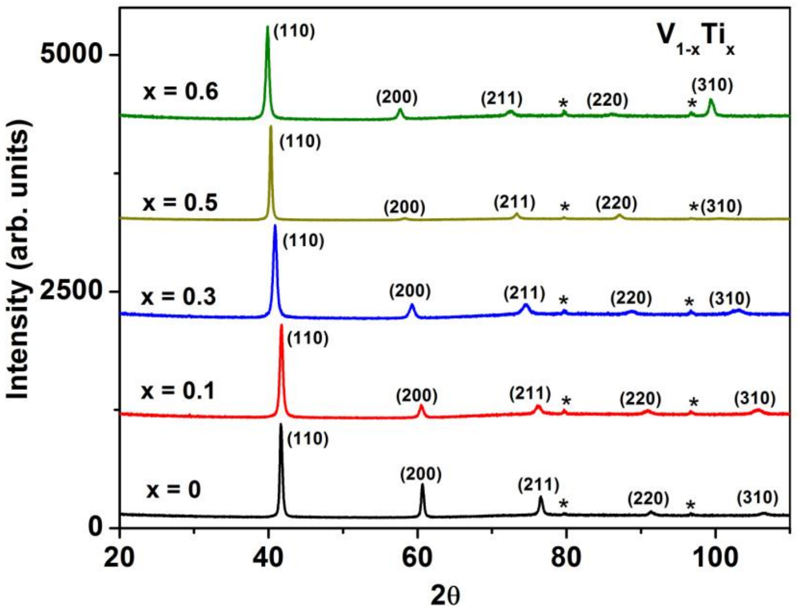


**Figure 1.** The X-ray diffraction patterns of the $V_{1-x}Ti_x$ alloys. The alloys were found to form in the body centred cubic phase.

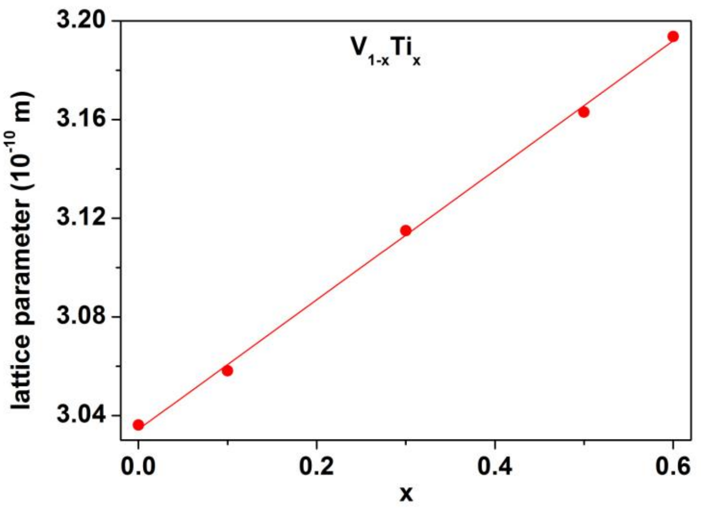


**Figure 2.** Variation of lattice parameter of the $V_{1-x}Ti_x$ alloys with Ti-concentration.

## ❖ Electrical resitivity:

The temperature dependence of electrical resistivity ($\rho(T)$) of the $V_{1-x}Ti_x$ alloys was measured in the temperature range 2-300 K in different magnetic fields using the AC Transport option of a 9 T physical properties measurement system (PPMS, Quantum design, USA). The electrical resistivity was measured using the four probe configuration. Figure 3 shows the temperature dependence of $\rho$ of the $V_{1-x}Ti_x$ alloys in the absence of magnetic field in temperature range 2-300 K. The $\rho(T)$ of V shows metallic character, with a residual resistivity ($\rho_0$) of 1.29 $\mu\Omega$-cm and a residual resistivity ratio (RRR = $\rho\ (300\ K)/\rho_0$) of 17.85. The $\rho_0$ increases and the RRR decreases with increasing Ti-content in the $V_{1-x}Ti_x$ alloys. For x = 0.6, the residual resistivity becomes 96.16 $\mu\Omega$-cm and the $\rho(T)$ becomes almost independent of temperature. As a result, the RRR drops to 1.07. All of these samples are superconducting at low temperatures. Figure 3(b) shows an enlarged view of $\rho(T)$ at temperatures below 8 K. When the temperature is reduced from the room temperature, V becomes superconducting below 5.22 K. The superconducting transition temperature ($T_c$) has been estimated as the temperature at which temperature derivative of $\rho(T)$ exhibits a maximum. The inset to figure 3(b) shows plot of ${}^{d\rho}/_{dT}$ as a function of temperature for V. The $T_c$ starts to increase as Ti is alloyed with V. For the present system, the $T_c$ increases till 30 atomic % of V is substituted by Ti, where it becomes 7.6 K. With further increase of the Ti-concentration, the $T_c$ slightly decreases and becomes 7.07 K for $V_{0.4}Ti_{0.6}$. The temperature dependence of $\rho$ and $T_c$ are commensurate with the previous measurements performed in our lab [3] and also to that reported in literature [4] for this alloy system. The electronic mean free path ($l_e$) can be estimated from the resistivity using the Sommerfeld theory of metals, where $l_e$ can be expressed in terms of the resistivity as [5],

$$l_e = \frac{(r_s/a_0)^2}{\rho} \times 92 \text{ Å} \tag{1}$$

where $r_s$ and $a_0$ are respectively radius of the sphere having volume equal to the volume per electron and Bohr radius and $\rho$ is the resistivity expressed in $\mu\Omega$-cm. Table 1 contains the $\rho_0$, RRR, $T_C$, $l_e$ and the lattice parameters for the present alloys.

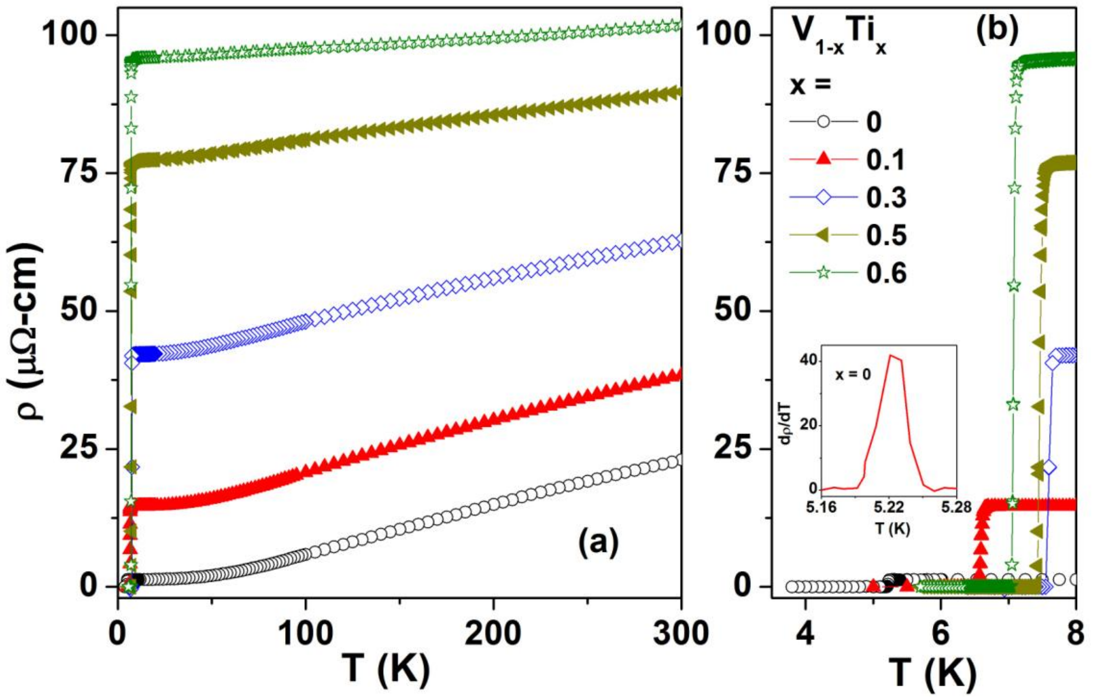


**Figure 3.** (a) Temperature dependence of $\rho(T)$ of the $V_{1-x}Ti_x$ alloys in the absence of magnetic field. As the Ti-content in V is increased, the $\rho_0$ increases and for x = 0.6, the $\rho(T)$ becomes almost independent of temperature. (b) Expanded view of $\rho(T)$ below 8 K in the absence of magnetic field.

**Table 1**

| % of Ti in V | $\rho_0$ ($\mu\Omega$-cm) | RRR | $T_C$ (K) (from $\rho$) | $l_e$ (Å) | $T_C$ (K) (from $\kappa$) | Lattice parameter (Å) |
|---|---|---|---|---|---|---|
| 0 | 1.311 | 17.85 | 5.22 | 193.64 | 5.162 | 3.0497 |
| 10 | 14.631 | 2.63 | 6.54 | 17.66 | 6.39 | 3.0581 |
| 30 | 42.159 | 1.50 | 7.6 | 6.54 | 7.33 | 3.1149 |
| 50 | 77.326 | 1.69 | 7.47 | 3.78 | 7.21 | 3.1629 |
| 60 | 96.156 | 1.07 | 7.07 | 3.15 | 7.02 | 3.1936 |

## ❖ Heat capacity:

The heat capacity of these alloys has been measured using the heat capacity option in the 9 T physical PPMS (Quantum design, USA), in the temperature range 2-20 K, in the normal and superconducting states. The heat capacity in the superconducting state was obtained in the absence of any applied magnetic field. The superconducting transition temperature ($T_c$) is defined as the temperature at which the temperature derivative of heat capacity shows a minimum. The normal state heat capacity for temperatures below $T_c$ was obtained by applying 8 T magnetic field. Some of these alloys has $H_{C2}$ greater than 8 T. For those alloys the normal state data has been obtained upto the temperature below which the sample becomes superconducting at 8 T. The normal state heat capacity of a material at low temperature ($T \ll \theta_D$) is given by,

$$C = \gamma T + \beta T^3, \tag{2}$$

where $\gamma T$ and $\beta T^3$ are respectively the electronic and phonon heat capacities. Using equation (2) we can separate the contribution from electrons and phonons to the heat capacity in the normal sate. Figure 4(a) shows the linear fit to $C/T$ vs $T^2$ for V. The intercept in the y-axis gives the value of $\gamma$ and the slope of the fitted curve gives $\beta$. Debye temperature for these alloys can be estimated from the heat capacity and is given as, $\theta_D = \sqrt[3]{\frac{1944.66}{\beta}}$. When a material becomes superconducting, the phononic contribution to the heat capacity remain same as that in the normal state but the electronic contribution changes due to formation of Cooper pairs. The formation of Cooper pairs depend on the superconducting energy gap ($\Delta$). Thus we get the idea about the superconducting energy gap from the electronic heat capacity in the superconducting state. The electronic heat capacity in the superconducting state ($C_{es}$) is obtained by subtracting the phonon heat capacity from the total heat capacity. The electronic heat capacity in the superconducting state is given as [6-8],

$$\frac{C_{es}}{\gamma T_C} = \frac{6\alpha^2}{\pi^2}\frac{1}{4\pi}\frac{T_C}{T}\int_0^{2\pi} d\emptyset \int_0^{\pi} d\theta sin\theta \int_0^{\infty} dx \left(-\frac{df}{dE}\right)\left(E^2 - \frac{T}{2}\frac{d\delta^2}{dT}\right), \tag{3}$$

where $E^2 = x^2 + \delta^2$, $f = \left(1 + \exp\left(\alpha T_c E/T\right)\right)^{-1}$ and $\alpha = \frac{\Delta(0)}{k_B T_c}$ . Here $\Delta(0)$ is the superconducting energy gap at absolute zero and $\delta = \frac{\Delta(0)}{\Delta(T)}$ . The estimated $\frac{\Delta(0)}{k_B T_c}$ for V is shown in figure 4(b). The empty circles in figure 4(b) shows the $\frac{C_{es}}{\gamma T_C}$ estimated experimentally and the red line corresponds to the theoretical estimation of the $\frac{C_{es}}{\gamma T_C}$ using equation (3). Here $\frac{\Delta(0)}{k_B T_c}$ is obtained as a fitting parameter, which is 1.78 for V. With increasing Ti-content in V, the $\frac{\Delta(0)}{k_B T_c}$ starts to increase and become 2.08 for $V_{0.5}Ti_{0.5}$. For x > 0.5, $\frac{\Delta(0)}{k_B T_c}$ decreases slightly and become 2.03.

This shows that these alloys are in the strong coupling limit. The jump in the heat capacity at $T_c$ $\left(\frac{\Delta C}{\gamma T_C}\right)$ also confirms this observation. Table 2 lists the various relevant parameters for the $V_{1-x}Ti_x$ alloys estimated from heat capacity.

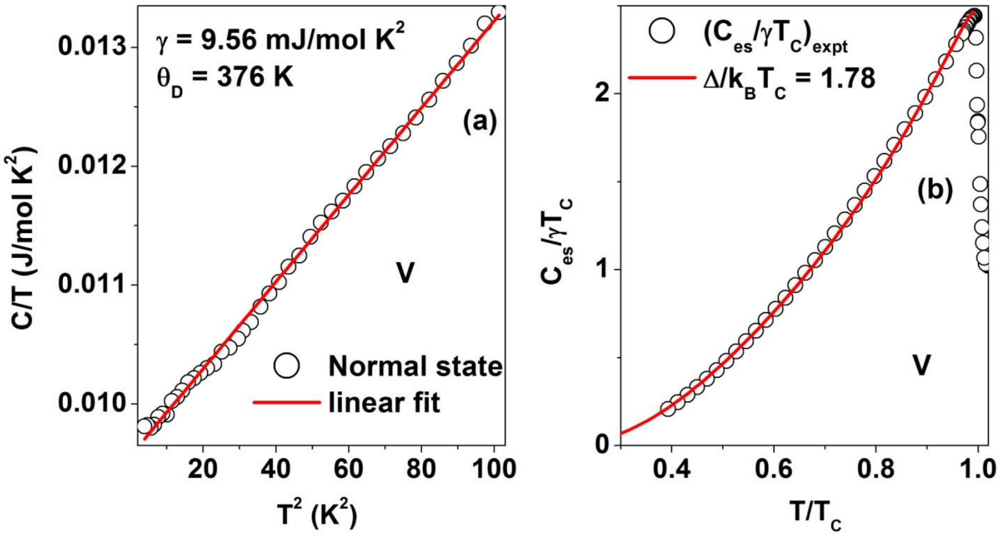


**Figure 4.** (a) Open circles are the $C/_T$ vs $T^2$ for V in the temperature range 2-10 K. The red line is the linear fit to the data. (b) Temperature dependence of $\frac{C_{es}}{\gamma T_C}$ as a function of $\frac{T}{T_c}$ for V. The red line is the theoretical $\frac{C_{es}}{\gamma T_C}$ for which fits the experimental values.

**Table 2:**

| x | $T_c$ (K) | $\gamma$ (J/mol K$^2$) | $\theta_D$ (K) | $\frac{\Delta C}{\gamma T_C}$ | $\frac{\Delta(0)}{k_B T_c}$ |
|---|---|---|---|---|---|
| 0 | 5.1 | 0.00956 | 376 | 1.498 | 1.78 |
| 0.1 | 6.41 | 0.01063 | 359 | 1.626 | 1.86 |
| 0.3 | 7.36 | 0.01098 | 326 | 1.881 | 1.97 |
| 0.5 | 7.05 | 0.01013 | 284 | 2.072 | 2.08 |
| 0.6 | 6.66 | 0.00971 | 265 | 2.087 | 2.03 |

## ❖ Thermal conductivity of the Ti-V alloys:

The thermal conductivity ($\kappa$) of $V_{1-x}Ti_x$ alloys has been measured using the thermal relaxation technique using the thermal transport option of the PPMS. Fig. 1(a) shows the $\kappa$ of the $V_{1-x}Ti_x$ alloys in the absence of magnetic field. The normal state thermal conductivity ($\kappa_n$) reduces drastically when 10 % of V is substituted by Ti. The $\kappa_n$ reduces further with increasing Ti-content in V. The peak observed in V around 38 K also disappears with the addition of Ti. The

thermal conductivity of V and some of the $V_{1-x}Ti_x$ alloys below $T_c$ in both the normal and superconducting states is shown in fig.1 (b)-(e). The $\kappa_n$ was obtained by applying up to 8 T magnetic field which is the highest field available in the present experimental set-up. The upper critical field for some of the present alloys is more than 8 T. The $\kappa_n$ for such alloys were obtained at temperatures ($T$) down to the onset of superconductivity in 8 T magnetic field. For V, the thermal conductivity in the superconducting state ($\kappa_s$) lies below the $\kappa_n$ due to the formation of Cooper pairs. For $V_{0.9}Ti_{0.1}$, the $\kappa_s < \kappa_n$ for $T < T_c$, though $\kappa_s$ shows a change of slope near 3 K. When 30% of V is substituted by Ti, the $\kappa_s$ starts increasing for $T < T_c$ and exhibits a maximum near 2.5 K. Even in the alloys with still higher Ti-concentration, the $\kappa_s$ is found to increase as the $T$ is lowered below the $T_c$. To analyze the normal state thermal conductivity, we have used the generalized expression for various scattering contributions that limits the thermal conductivity in a metal. Electronic thermal resistivity limited by electron-defect scattering ($\omega_{e-d}$) and electron-phonon scattering are given as [9],

$$\omega_{e-d} = \frac{A_{e-d}}{T} \qquad (4)$$

and

$$\omega_{e-ph} = \frac{B_{e-l}}{T}\left(\frac{T}{\theta_D}\right)^5 J_5\left(\frac{\theta_D}{T}\right)\left\{1 + \frac{3}{\pi^2}\left(\frac{k_F}{q_D}\right)^2\left(\frac{\theta_D}{T}\right)^2 - \frac{1}{2\pi^2}\frac{J_7\left(\frac{\theta_D}{T}\right)}{J_5\left(\frac{\theta_D}{T}\right)}\right\}. \qquad (5)$$

Here $\theta_D$ is the Debye temperature. The function $J_n\left(\frac{\theta_D}{T}\right)$ is given by,

$$J_n\left(\frac{\theta_D}{T}\right) = \int_0^{\frac{\theta_D}{T}} \frac{x^n e^x}{(e^x-1)^2}\, dx. \qquad (6)$$

The phononic thermal conductivity is given as [10],

$$\kappa_{ln} = MT^3 \int_0^{\infty} du \frac{u^4 e^u}{(e^u-1)^2} \frac{1}{N + \frac{CuT}{J_3\left(\frac{\theta_D}{T}\right)} + LuT + Pu^4T^4} \quad , \qquad (7)$$

here $N$, $C$, $L$ and $P$ are respectively scattering coefficients due to phonon scattering from grain boundaries, electrons, dislocations and point defects respectively, whereas $u = \frac{\hbar\omega}{k_B T}$ is the reduced phonon energy and the constant $M = \frac{{k_B}^4}{2\pi^2\hbar^3 v_s}$.

Now as the material becomes superconducting, the normal electrons reduce due to the formation of Cooper pairs. Thus the electronic thermal conductivity in the superconducting state will change. The phononic contribution to the thermal conductivity in the superconducting state will also change due to reduction in phonon scattering from electrons. These changes in the electronic and phononic thermal conductivities in the superconducting state are given by the Bardeen-Rickayzen-Tewordt (BRT) theory of thermal conductivity of superconductors. According to the BRT theory, the ratio of the superconducting state thermal conductivity to the normal state thermal conductivity limited by electron-defect scattering is given by [11],

$$\left(\frac{\kappa_s}{\kappa_n}\right)_{e-d} = \frac{1}{f(0)}\left[f(-y) + yln(1+\exp(-y)) + \frac{y^2}{2(1+\exp(y))}\right]. \quad (8)$$

Here $y = \frac{\Delta(T)}{k_B T}$ and $f(-y)$ is the Fermi integral given by, $f(-y) = \int_0^\infty \frac{zdz}{1+\exp(z+y)}$ .

Again, the ratio of the superconducting state thermal conductivity to the normal state thermal conductivity limited by electron-phonon scattering is given by [12],

$$\left(\frac{\kappa_s}{\kappa_n}\right)_{e-ph} = \frac{\int_1^\infty dx\, x(x^2-1)^{1/2} sech^2\left(\frac{1}{2}xy\right)[\Gamma_s(xy)]^{-1}}{\int_0^\infty dz\, z^2 sech^2\left(\frac{1}{2}z\right)[\Gamma_n(z)]^{-1}}. \quad (9)$$

Here $y$ has similar meaning as before and $\Gamma_s(xy)$, $\Gamma_n(z)$ are defined as,

$$\Gamma_s(xy) = \int_0^{x-1} \frac{dt\, t^2(x-t-x^{-1})}{[(x-t)^2-1]^{1/2}}\left\{\left(1+e^{-y(x-t)}\right)^{-1} + (e^{yt}-1)^{-1}\right\}$$
$$+ \int_0^\infty \frac{dt\, t^2(x+t-x^{-1})}{[(x+t)^2-1]^{1/2}}\left\{(1-e^{-yt})^{-1} - \left(1+e^{-y(x+t)}\right)^{-1}\right\}$$
$$+ \int_{x+1}^\infty \frac{dt\, t^2(t-x+x^{-1})}{[(t-x)^2-1]^{1/2}}\left\{(1+e^{y(t-x)})^{-1} + (e^{yt}-1)^{-1}\right\} \quad (10)$$

and $\Gamma_n(z) = \left(8/3\right)F_2(0) + F_2(z) + F_2(-z)$ (11)

where $F_2(z)$ is defined as,

$$F_2(z) = \int_0^\infty dt\, t^2(1+e^{t-z})^{-1} \quad (12)$$

The phononic contribution to thermal conductivity in the superconducting state is given by [13],

$$\kappa_{ls} = MT^3 \int_0^\infty du \frac{u^4 e^u}{(e^u-1)^2} \frac{1}{N + \frac{CuTg(u)}{J_3\left(\frac{\theta_D}{T}\right)} + LuT + Pu^4T^4} \quad . \quad (13)$$

The function $g(u)$ gives the change in phonon-electron scattering due to the formation of Cooper pairs. The functional form of $g(u)$ is given as [11],

$$g(u) = \frac{1-e^{-u}}{u}(2J_1 + J_2), \quad (14)$$

where $J_1 = \int_{\Delta(0)}^\infty dE\left(\frac{\epsilon^2+Eu}{\epsilon\epsilon'}\right)f(E)f(-E')$ and $J_2 = \int_{-u+\Delta(0)}^{-\Delta(0)} dE\left|\frac{EE'}{\epsilon\epsilon'}\right|\left(1-\frac{(\Delta(0))^2}{EE'}\right) f(E)f(-E')$.

$\Delta(0)$ is the superconducting energy gap at $T=0$ and $E'$ is defined as $E' = E+u$. $E$ and $f(E)$ are defined as, $E^2 = \epsilon^2 + (\Delta(T))^2$ and $f(E) = \frac{1}{1+e^{E/k_BT}}$ .

For analyzing the thermal conductivity results, all these integrations were evaluated numerically using Matlab.

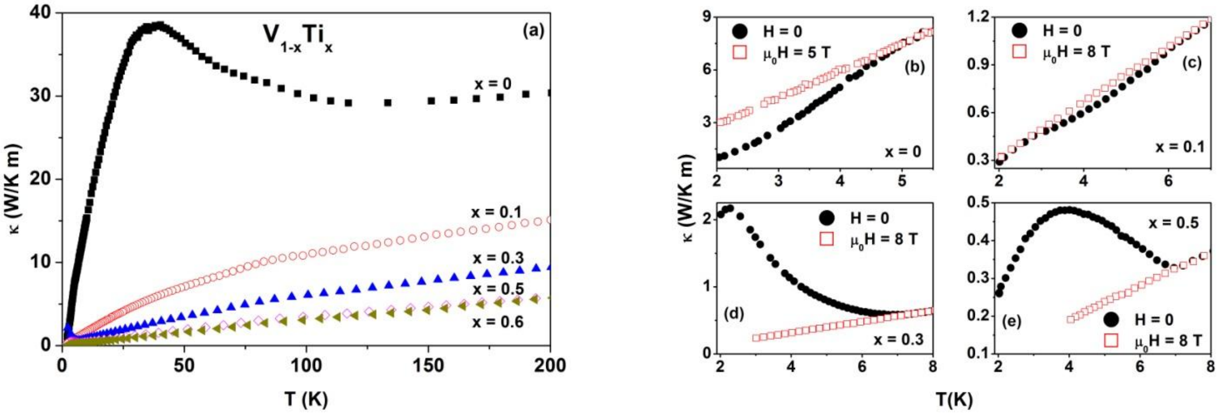


**Figure 5.** (a): Thermal conductivity ($\kappa$) of the $V_{1-x}Ti_x$ alloys in the absence of magnetic field. (b) – (e): The $\kappa$ of V and some of the $V_{1-x}Ti_x$ alloys in the normal and superconducting states.

## References:


1. Ch. Leibovitch et al, Metallurgical Transactions A **12A**, 1513 (1981).
2. G. Aurelio et al, Metallurgical and Materials Transactions A **33A**, 1303 (2002).
3. Md. Matin, L. S. Sharath Chandra, S. K. Pandey, M. K. Chattopadhyay, and S. B. Roy, Eur. Phys. J. B **87** 131 (2014).
4. V. A. Rassokhin, N. V. Volkenshtein, E. P. Romanov, and A. F. Prekul, Sov. Phys.-JETP **39** 166 (1974) [Zh. Eksp. Teor. Fiz. **66** 348 (1974)].
5. See, e.g., N. W. Ashcroft and N. D. Mermin, "*Solid State Physics*" (Cengage Learning India Pvt. Ltd., Delhi India 2015), pp. 52.
6. Shyam Sundar, L. S. Sharath Chandra, M. K. Chattopadhyay, and S. B. Roy, J. Phys.: Condens. Matter **27** 045701 (2015).
7. H. Padamsee, J. E. Neighbor, and C. A. Shiffman, J. Low Temp. Phys. **12** 387 (1973).
8. C L. Huang, J-Y Lin, C. P. Sun, T. K. Lee, J. D. Kim, E. M. Choi, S. I. Lee, and H. D. Yang, Phys. Rev. B **73** 012502 (2006).
9. "*Thermal Conductivity Theory, Properties and applications*", ed. T.M. Tritt, (Kluwer Academic / Plenum Publishers, New York 2004).
10. P. H. Kes, J. G. A. Rolfes, and D. de Klerk, J. Low Temp. Phys. **17** 341 (1974).
11. J. Bardeen, G. Rickayzen, and L. Tewordt, Phys. Rev. **113** 982 (1959).
12. L. Tewordt, Phys. Rev. **128** 12 (1962).
13. L. Tewordt, and Th. Wölkhausen, Solid State Comm. **70** 839 (1989).
